# Supplementary material for: D2D Assisted Beamforming for Coded Caching
Source: arXiv:1905.05446 source file (2019-05-14)
Supplement: Supplementary file 1 [file appendix.tex]

\appendices
\section{Proof of Theorem 1}
\label{sec:app}

Consider the case when no D2D transmission is available, in this case the total number of massages ($\tilde{X}^{\mathcal{S}}_{\mathcal{T}}$) that should be transmitted to all the users is $\mathbf{M}_{\text{T}}=\binom{t+L}{t+1}$, and each user needs $\binom{t+L-1}{t}$ number of these massages to decode its intended file. Thus, the total number of MAC conditions that should be considered for each user is $2^{\binom{t+L-1}{t}}-1$. Therefore, the total number of MAC conditions that should be taken care of in beam design for all the users is $(t+L)(2^{\binom{t+L-1}{t}}-1)=\text{MAC}_{\text{Total}}$.

Now assume that $i$ number of D2D time slots has happened, in this case, depending on which subsets are selected, there will be different number of MAC conditions in beam design. When single D2D time slot happens, the users that are included in that subset ($S_{1}$), receive one of their intended massages in the D2D sub-phase. Therefore, in the DL-phase the BS eliminates that massage from the transmitting signal and sends the rest of the massages. Moreover, the users that were involved in D2D transmission require one less number of massages to decode their data. Thus, the number of MAC conditions for these users decreases to almost half ($\frac{2^{\binom{t+L-1}{t}-1}-1}{2^{\binom{t+L-1}{t}}-1}=\frac{\beta_{2}}{\beta_{1}}  \approx  0.5$) and the total number of MAC conditions decreases to $(L-1)(2^{\binom{t+L-1}{t}}-1)+(t+1)(2^{\binom{t+L-1}{t}-1}-1)=\text{MAC}_{\text{Total}}-(t+1)0.5\beta_{1}$. 

Now consider that another D2D transmission happens, assume that this one happens among $t+1$ different users ($S_{2},\ S_{1} \cap S_{2}= \emptyset$). Therefore, the total number of MAC conditions further decreases to $(L-(t+2))(2^{\binom{t+L-1}{t}}-1)+2(t+1)(2^{\binom{t+L-1}{t}-1}-1)=\text{MAC}_{\text{Total}}-2(t+1)0.5\beta_{1}$. However, if $|S_{1} \cap S_{2}|= \alpha$, instead of decreasing the total number of MAC condition by $0.5\alpha \beta_{1}$, the total number of MAC conditions will be decreased by $0.5\alpha \beta_{2}$ for this number of users, which is the half  ($\frac{\alpha \beta_{2}}{\alpha \beta_{1}} \approx 0.5$) of the case $\ S_{1} \cap S_{2}= \emptyset$. 

Thus, in general when the number of D2D transmissions occur uniformly among all the users the total number of MAC condition is minimum. In other word, when the difference between the maximum number of MAC conditions and the minimum number of MAC conditions is the least the number of MAC conditions is minimum. On the other hand, when the number of D2D transmissions occur for limited number of users, the number of MAC conditions is maximum. 

\subsection{minimum number of MAC conditions}
The total number of massages that BS should deliver to all the users (after $i$ number of D2D time slots) is $\binom{t+L}{t+1}-i$. Moreover, each of these massages contains $t+1$ number of fragments, thus, the total number of fragments that BS must send to all the users is $(t+1)(\binom{t+L}{t+1}-i)$. According to the previous paragraph, when these fragments are distributed uniformly among all the users the total number of MAC conditions is minimum in beam design. Therefore, when the fraction $a=\frac{(t+1)(\binom{t+L}{t+1}-i)}{t+L}$ is integer, all the users receive $a$ number of fragments to decode their files. However when $a$ is not integer, ($t+L-b$) number of users receive $a=\left\lfloor{\frac{(t+1)(\binom{t+L}{t+1}-i)}{t+L}}\right\rfloor$ number of file fragments and $b$ number of users receiver $a+1$ number of file fragments ($b$ is defined in \eqref{eq:NA2}). Thus, the minimum number of MAC conditions after $i$ D2D time slots is:
\begin{equation} \nonumber
    \text{MAC}^{i}_\text{min} =(t+L-b)(2^a-1)+b(2^{a+1}-1)
\end{equation}

\subsection{maximum number of MAC conditions}
Consider that $i$ number of D2D times lots are done, as discussed earlier, when these number of D2D transmissions occur among a limited number of users, the number of MAC conditions is larger. Thus, the minimum number of users that is required for $i$ number of different D2D subsets is $U$, which is defined as following
\begin{equation} \nonumber
    \binom{U-1}{t+1} <  i\leqslant \binom{U}{t+1}\nonumber
\end{equation}

Now since the negative of the derivative of the function $2^{x-i}$ is monotonically decreasing with respect to $i$, the decrement in the amount of the function is smaller for the larger amount of $i$. %Thus, the worst situation happens when all the subsets of size $t+1$ are chosen for $U-1$ number of users, and the rest of the subsets must be chosen from those $U-1$ users and a new user. 
Moreover, according to the previous discussions, when D2D transmissions occur among limited number of users the total number of MAC conditions is maximum. Therefore, when for $U-1$ number of users all the subsets of size $t+1$ are chosen and the rest of the subsets are chosen from $t$ number of these users and a new user, the total number of MAC conditions is maximized. Thus, the number of subsets in which the new user must be presented is
\begin{equation} \nonumber
    X=i  -\binom{U-1}{t+1}
\end{equation}

To fulfil this extra $X$ D2D time slots, the remaining subsets of users (of a size $t+1$) are consist of a new user and $t$ users from the previous group. Again when these new subsets are chosen from the limited number of users, the number of MAC conditions is larger. Thus, the minimum number of users (form the previous group) that are needed to form the new subsets, is $U_{1}$ and is defined as
\begin{equation} \nonumber
    \binom{U_{1}-1}{t} <  X\leqslant \binom{U_{1}}{t}
\end{equation}

Therefore in this types of scenarios we have 4 different types of users\\
1) Those who doesn't receive any file fragment in D2D transmissions. So they need $\binom{t+L-1}{t}$ number of file fragments in DL transmission and their total number is $t+L-U$.\\
2) those who has received all the available file fragments from D2D transmissions in subsets consisting of $U-1$ number of users, but did not receive any file fragments in subsets consisting of a new user. Thus, they need $\binom{t+L-1}{t}-\binom{(U-1)-1}{t}$ number of file fragments in DL transmission and their total number is $U-(U_{1}+1)$\\
3) one new user who has received $X$ number of file fragments in the new subsets consisting of it self and $U_{1}$ number of other users. Thus, it needs $\binom{t+L-1}{t}-X$ number of file fragments in DL transmission.\\
For the fourth type of users whose total number is $U_{1}$ the number of needed file fragments in DL transmission is a little bit tricky. First they have received all the file fragments from other $U-2$ number of users in the previous user group (of size $U-1$) and they have received some file fragments in new groups. If $X=\binom{U_{1}}{t}$ all of them will receive another $\binom{U_{1}-1}{t-1}$ number of file fragments in new subsets. However, if $Y=\binom{U_{1}}{t}-X$ is not equal to zero, based on the subset selection we will again have different types of users inside this type of users. Thus, in order to avoid more complicated upper bound and to be able to state something in general, we assume that all of these users receive another $\binom{U_{1}-1}{t-1}-Y$ number of file fragments in these new D2D transmissions. Therefore, the upper bound is not tight in all scenarios but its is tight enough. 

Therefore, the maximum number of MAC conditions after $i$ D2D time slots is less or equal to
\begin{align} 
        &\text{MAC}^{i}_\text{max}=(t+L-U)(2^{\binom{t+L-1}{t}}-1)+&\nonumber\\&(U-(U_{1}+1))(2^{(\binom{t+L-1}{t}-\binom{U-2}{t})}-1)+& \nonumber \\
    &U_{1}(2^{(\binom{t+L-1}{t}-(\binom{U-2}{t}+\binom{U_{1}-1}{t-1}-Y))}-1)+& \nonumber \\&(2^{\binom{t+L-1}{t}-X}-1)\text{,}\nonumber&
\end{align}
