# Supplementary material for: D2D Assisted Beamforming for Coded Caching
Source: arXiv:1905.05446 source file (2019-05-14)
Supplement: Supplementary file 2 [file appendixB.tex]

\section{Proof of Theorem 2}
\label{sec:appB}
\begin{figure}
    \centering 
    \includegraphics[width=1\columnwidth,keepaspectratio]{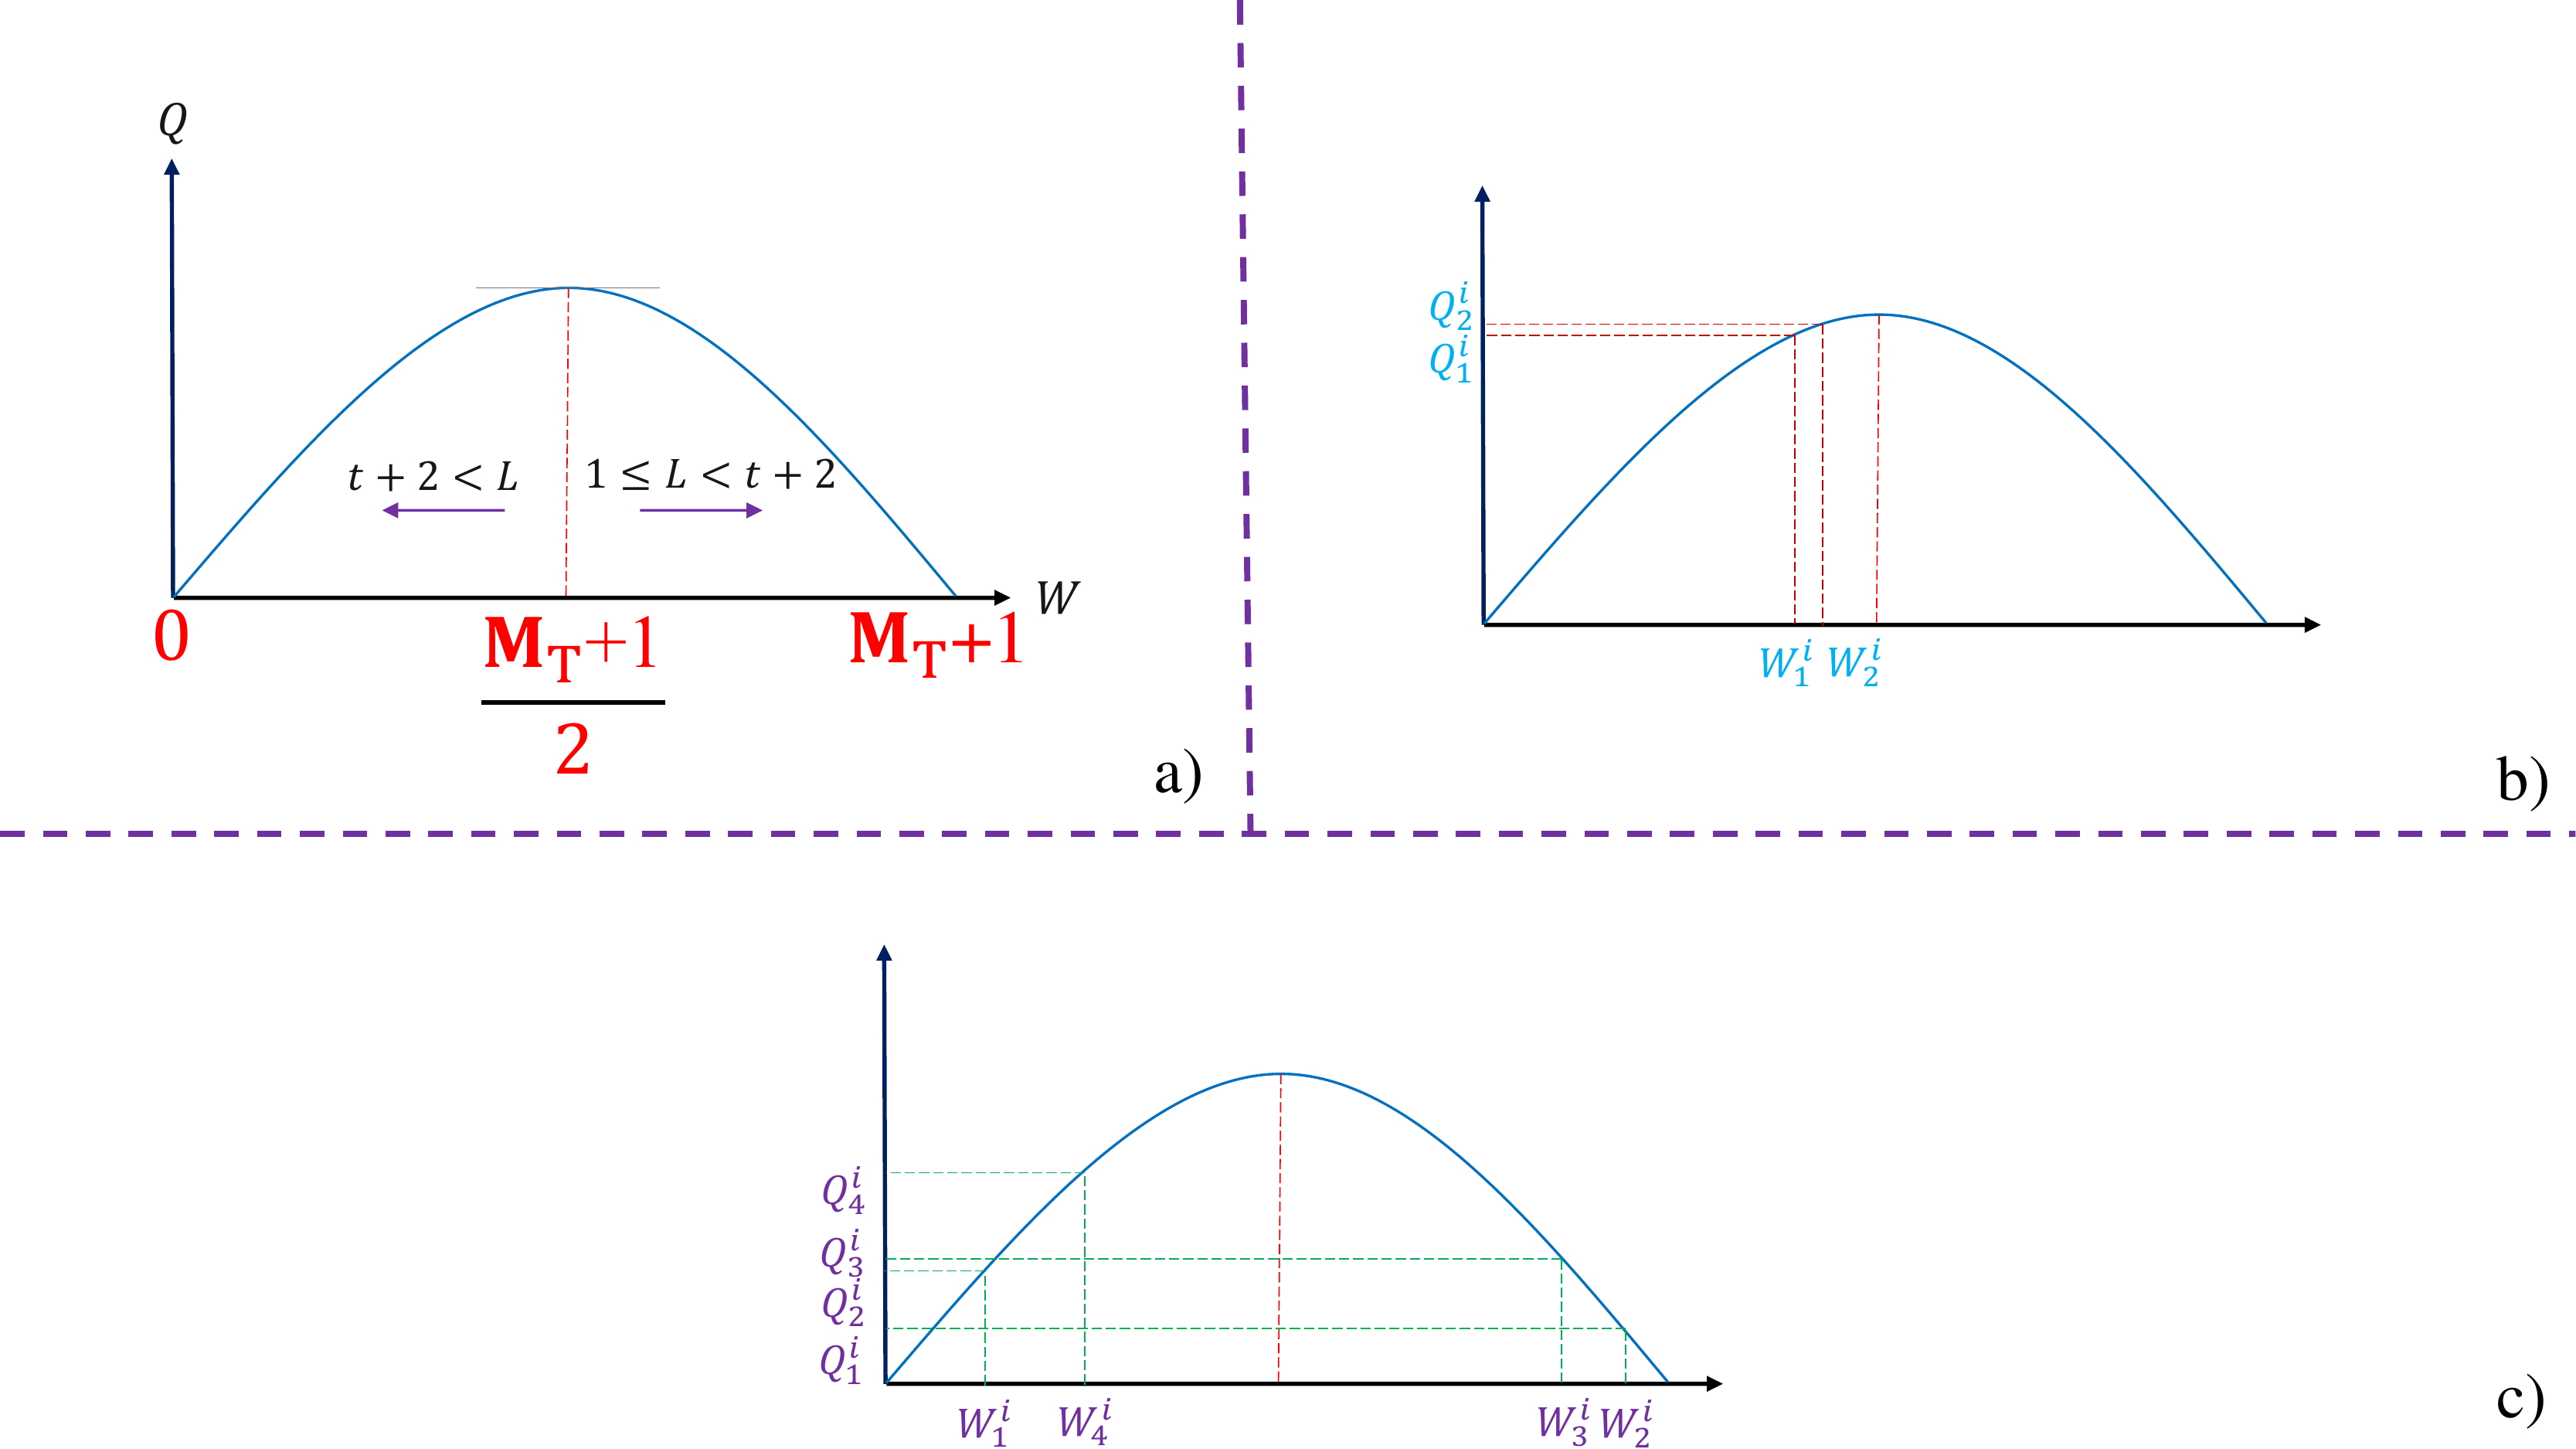}
    \caption{Total number of quadratic variables for each user in different scenarios. a) general behavior b) uniform scenario c)limited number of users scenario. Figure (b) and (c) show the needed massages $W^{i}_{k}$ and corresponding total quadratic equations $Q^{i}_{k}$ for different types of users in two extreme cases.}
\label{fig:quadbehav}
\end{figure}
In general, when D2D transmissions are not available, the BS must send $\mathbf{M}_{\text{T}}=\binom{t+L}{t+1}$ total number of massages. Moreover, each user needs $W=\binom{t+L-1}{{t}}$ number of these massages, therefore, each user sees the rest of the massages ($\mathbf{M}_{\text{T}}-W$) as interference. Furthermore, for each of needed massages the BS must consider ($\mathbf{M}_{\text{T}}-W+1$) number of quadratic variables in conditions like \eqref{prob:dlprob_ex2} for each user. Thus, for each user, the BS must consider $Q=W(\mathbf{M}_{\text{T}}-W+1)$ number of quadratic variables in its' beamformers.

The total number of quadratic variables $Q$ is a second order polynomial on $W$ (see Fig. \ref{fig:quadbehav} (a)), which is maximum when $W$ is $\frac{\mathbf{M}_{\text{T}}+1}{2}$. On the other hand, $W$ is equal to $\frac{t+1}{t+L}\mathbf{M}_{\text{T}}$, Thus when $1 \leq L < t+2$, $W$ is on the right hand  side of the maximum point and when $t+2 < L$ it is on the left hand side of it.

When $i$ number of D2D time slots has happened, based on which D2D subsets have been chosen for D2D transmission $W^{i}_{k}$ (the total number of needed messages for a particular user after $i$ D2D time slots) and $\mathbf{M}^{i}_{\text{T}}$ (the total number of massages that is sent by BS after $i$ number of D2D time slots are done) can have any relation ($0 \leq \frac{W^{i}_{k}}{\mathbf{M}^{i}_{\text{T}}} \leq 1$).

Now two extreme cases are important, when the D2D transmission happen uniformly among all the users and when it happens among limited number of user (as it is discussed in Appendix A). For the first case, since all the users have received almost the same number of file fragments in D2D sub-phase, in DL sub-phase they all need almost a same fraction of the total transmitted massages ($\mathbf{M}^{i}_{\text{T}}$). On the other hand, in second scenario, since a limited number of users have received most of their intended files in D2D sub-phase, they need a few number of massages in $\mathbf{M}^{i}_{\text{T}}$ to decode their files. Further more, those users who haven't been in any D2D transmission, need most of the files, thus in this types of scenarios users are either on the right hand side of the maximum point or on the left hand side of it. Fig. \ref{fig:quadbehav} (b) and (c) show the extreme cases for particular $t$ and $L$.

Therefore, these two cases are also two extreme cases for total number of quadratic variables too. In this manner, when D2D subsets are chosen uniformly among all the users, the total number of quadratic variables is maximized since all the users' needed massages ($W^{i}_{k}$) are close to the maximum point($\frac{\mathbf{M}^{i}_{\text{T}}+1}{2}$). On the other hand, when limited number of users are chosen for D2D transmissions, $Q$  is minimized since users' needed massages are either on the left hand side of the maximum point or on the right hand side of it.

Therefore, the total number of quadratic variables for all the users after $i$ number of D2D time slots is computed as \\
\begin{equation} \nonumber    
Q^{i}=\sum_{k \in [K]}Q^{i}_{k}
\end{equation}
where 
\begin{equation} \nonumber
    Q^{i}_{k}=W^{i}_{k}(\mathbf{M}^{i}_{\text{T}}-W^{i}_{k}+1)
\end{equation}

By using the total number of needed massages for each user defined in appendix A, equations \eqref{eq:NA9} and \eqref{eq:NA11} is achieved.
